# Supplementary material for: Improving Robustness of Learning-based Autonomous Steering Using Adversarial Images
Source: arXiv:2102.13262 source file (2021-02-26)
Supplement: Supplementary file 1 [file 7-appendix.tex]

% \begin{table}[ht]
%   \caption{Mean Accuracy correlation 2}
%   \label{tb:style_driving_unit}
%   \centering
%   \begin{tabular}{c|cccc}
%     \toprule
%     \multicolumn{1}{c}{} & \multicolumn{4}{c}{Test} \\
%     \cmidrule(r){2-5}
%     \multicolumn{1}{c}{Train} &  \vBase{}& \vrgan{} & \vrmunit{} & \rBase{}\\
%     \midrule
%             \vBase{} & 53.72\% & 43.43\% & 28.00\% & 31.16\%\\
%             \vrgan{} & 33.76\% & 50.02\% & 33.71\%  & 26.87\%\\
%             \vrmunit{} & 31.29\% & 25.69\% & 39.99\% & 25.56\% \\
%             \rBase{} & 41.42\% & 52.43\%  & 44.79\%   & 88.36\%\\
%     \bottomrule
%   \end{tabular}
% \end{table}


% \begin{figure}[h]
% \begin{center}
%   \includegraphics[width=\linewidth]{figures/distribution.png}
% \end{center}   
% \caption{Steering angle distribution of NVIDIA (real) and Udacity (virtual) datasets.}
% \label{fig_driving_data_distribution}
% \end{figure}


% \begin{comment}
% \subsubsection{Experiment 1 results and analysis}
% \begin{table}[ht]
%   \caption{Mean Accuracy comparison of driving tasks in different image qualities (\%)}
%   \label{tab_quality_driving_unit}
%   \centering
%   \begin{tabular}{c|cccccccccc}
%     \toprule
%     \multicolumn{1}{c}{} & \multicolumn{10}{c}{Test}                   \\
%     \cmidrule(r){2-11}
%     \multicolumn{1}{c}{Train} & R & B1 & B2 & B3 & N1 & N2 & N3 & D1 & D2 & D3 \\
%     \midrule
%             R & 88.36 & 88.21 & 88.06 & 86.07 & 88.33 & 86.01 & 81.42 & 88.30 & 88.63 & 74.97 \\
%             \bOne{} & 87.05 & 87.08 & 86.84 & 83.98 & - & - & - & - & - & - \\
%             \bTwo{} & 89.10 & 89.16 & 89.34 & 86.42 & - & - & - & - & - & - \\
%             \bThree{} & 86.16 & 86.16 & 85.74 & 87.70 & - & - & - & - & - & -  \\
%             \nOne{} & 89.10 & - & - & - & 88.45 & 86.54 & 81.16 & - & - & -  \\
%             \nTwo{} & 86.57 & - & - & - & 87.50 & 87.35 & 83.54 & - & - & -  \\
%             \nThree{} & 66.63 & - & - & - & 66.72 & 66.19 & 66.22 & - & - & -  \\
%             \dOne{} & 88.06  & - & - & - & - & - & - & 88.09 & 87.76 & 72.70  \\
%             \dTwo{} & 88.60  & - & - & - & - & - & - & 88.95 & 88.92 & 75.14  \\
%             \dThree{} & 75.56  & - & - & - & - & - & - & 75.62 & 76.75 & 89.01  \\
%     \bottomrule
%   \end{tabular}
% \end{table}
% \end{comment}


\clearpage
\section{Appendix}
In this section, we explore the relationship between the batch normalization statistics difference and the Mean Accuracy difference in our task, from the perspectives of image quality and image style.

\subsection{Analysis of Batch Normalization Statistics}
% Let $MR=train(R)$ represent the model trained on \rBase{}, and similarly $MV=train(V)$. We split \rBase{} into $trainR$ and $testR$, and split \vBase{} into $trainV$ and $testV$, with $train:test \approx 10:1$.


%According to the experiments, the result of training on R and testing on R is 88.36\%, while training on V and testing on R is only 31.16\%. 
%Our hypothesis is, $BN(MR, trainR)$ is similar with $BN(MR, testR)$, and $BN(MV, trainV)$ is not similar with $BN(MV, testR)$, and $BN(MV, testR)$ is not similar with $BN(MR, testR)$.

Here, we present the analysis of batch normalization (\BN{}) statistics of our experiments. The learning algorithm we consider (from Bojarski et al.~\cite{bojarski2016end}) consists of five convolutional layers followed by three fully-connected layers, and has the following specifications. 

\begin{itemize}
    \item Input layer output: 3 dimensions (RGB channels); 
    %normalize images from $[0,255]$ to $[-1,1]$;
    \item Convolutional layer 1 output: 24 dimensions (feature maps);
    \item Convolutional layer 2 output: 36 dimensions (feature maps);
    \item Convolutional layer 3 output: 48 dimensions (feature maps);
    \item Convolutional layer 4 output: 64 dimensions (feature maps);
    \item Convolutional layer 5 output: 64 dimensions (feature maps);
    \item Fully-connected layer 1 output: 1 dimension;
    \item Fully-connected layer 2 output: 1 dimension;
    \item Fully-connected layer 3 output: 1 dimension; and
    \item Output layer output: 1 dimension. 
\end{itemize}



We record the \BN{} statistics of all layers. If a layer has a nonlinear activation, the \BN{} statistics are collected before the application of the activation function. We calculate the mean and standard deviation of each dimension. As a result, we have 3 + 24 + 36 + 48 + 64 + 64 + 1 + 1 + 1 + 1 = 243 mean values and 243 standard deviation values. 

We use $\rm{train}(A)$ to denote the model trained on $A$, and \BNMD{$M$}{B} to denote the \BN{} statistics of dataset $B$ on the model $M$. Specifically, we use \BN{}$^{mean}$ to denote the mean vector of the \BN{} statistics, and \BN{}$^{std}$ to denote the standard deviation vector of the \BN{} statistics. In this section, we mainly consider the \ltwo{} norm of either the mean values or the standard deviation values of one set of \BN{} statistics to the other set of \BN{} statistics. In particular, we denote by ${\rm{BN}}^{mean}$ and ${\rm{BN}}^{std}$ the mean and standard deviation vectors of \BN{}, respectively. In addition, we use the \BN{} statistics of ${\rm{BN}}_{R_{test}}($\train$(R_{train}))$ as our baseline to be compared with, where $R_{train}$ and $R_{test}$ indicate the training set and test set of $R$, respectively.



\begin{figure}[h]
\begin{center}
  \includegraphics[width=\textwidth]{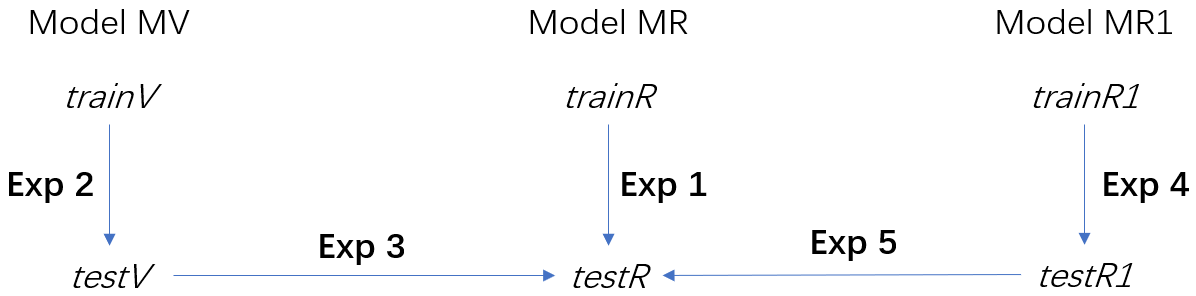}
\end{center}   
\caption{Relationships of the 5 comparison experiments. Model MV is trained on the virtual dataset Udacity, Model MR is trained on the real dataset Nvidia, and model MR1 is trained on another real dataset Honda.}
\label{fig:BN_ratio_RR}
\end{figure}




\subsection{Layer-by-layer Batch Normalization Statistics Analysis}
We do layer-by-layer batch normalization statistics analysis to show the difference of the model training on R and V. Let MR=train($R_{train}$), and MV=train($V_{train}$). We will show the layer-by-layer BN statistics difference between trainR and testR on model MR (comparison 1), trainV and testV on model MV (comparison 2), and testV and testR on model MV (comparison 3).

For comparison 1, we show the results in Table~\ref{tb:appdixA_exp1} and Fig~\ref{fig:BN_ratio_RR}. Since it's trained and tested on the same dataset R, the differences are relatively small (1.86\% for mean and 0.72\% for std in model-level). 

%in layer-level and model-level.

%Let (A, B) represent the process of training on dataset A and testing on dataset B.


% \begin{figure}[h]
% \begin{center}
%   \includegraphics[width=\linewidth]{figures/exp_relation.jpg}
% \end{center}   
% \caption{The relationship of 3 experiments.}
% \label{fig:exp_relation}
% \end{figure}

%\subsection{Baseline}


% Verify $BN(MR, trainR)$ is similar with $BN(MR, testR)$.

% From Table \ref{tb:appdixA_exp1}, we can find the differences of mean and std are small.


% \begin{table}[ht]
%   \caption{L2 norms of mean and standard deviation of \BNDDC{$trainR$}{testR}{}}
%   \label{tb:appdixA_exp1}
%   \centering
%   \scalebox{0.8}{
%   \begin{tabular}{c|ccccccccccc}
%     \toprule
%     BN Position & Input & Conv1 & Conv2 & Conv3 & Conv4 & Conv5 & FC1 & FC2 & FC3 & Output & Model level\\
%     \midrule
%     $\|$\BNDDC{$trainR$}{testR}{mean}$\|_2$ & 0.093 & 0.992 & 6.416 & 28.22 & 20.68 & 19.86 & 0.294 & 0.392 & 1.865 & 0.093 & 40.80 \\
%     $\|$\BNDDC{$trainR$}{testR}{std}$\|_2$ & 0.555 & 3.453 & 14.66 & 41.43 & 60.17 & 53.53 & 5.124 & 2.485 & 2.594 & 1.604 & 92.04 \\
%     \bottomrule
%   \end{tabular}
%   }
% \end{table}

%\clearpage{}

\begin{table}[ht]
  \caption{L2 norms of BN mean and standard deviation for dataset trainR and testR on Model MR, and their differences. MA(MR, trainR)=95.33\%, MA(MR, testR)=88.36\%.}
  \label{tb:appdixA_exp1}
  \centering
  \scalebox{0.7}{
  \begin{tabular}{c|ccccccccccc}
    \toprule
    BN Position & Input & Conv1 & Conv2 & Conv3 & Conv4 & Conv5 & FC1 & FC2 & FC3 & Output & Model level\\
    \midrule
    mean trainR & 0.092 & 0.987 & 6.387 & 28.13 & 20.49 & 19.61 & 0.298 & 0.388 & 1.864 & 0.107 & 40.52 \\
    mean testR & 0.093 & 0.992 & 6.416 & 28.22 & 20.68 & 19.86 & 0.294 & 0.392 & 1.865 & 0.093 & 40.80 \\
    mean diff & 0.001 & 0.008 & 0.045 & 0.191 & 0.361 & 0.491 & 0.004 & 0.004 & 0.001 & 0.014 & 0.754 \\
    mean diff / mean trainR & 1.09\% & 0.81\% & 0.70\% & 0.68\% & 1.76\% & 2.50\% & 1.34\% & 1.03\% & 0.05\% & 13.08\% & 1.86\% \\
    \midrule
    std trainR & 0.553 & 3.444 & 14.63 & 41.37 & 60.10 & 53.53 & 5.143 & 2.495 & 2.601 & 1.740 & 91.97 \\
    std testR & 0.555 & 3.453 & 14.66 & 41.43 & 60.17 & 53.53 & 5.124 & 2.485 & 2.594 & 1.604 & 92.04 \\
    std diff & 0.001 & 0.009 & 0.032 & 0.115 & 0.229 & 0.433 & 0.018 & 0.010 & 0.007 & 0.136 & 0.662 \\
    std diff / std trainR & 0.18\% & 0.26\% & 0.22\% & 0.28\% & 0.38\% & 0.81\% & 0.35\% & 0.40\% & 0.27\% & 7.82\% & 0.72\% \\
    \bottomrule
  \end{tabular}
  }
\end{table}

\begin{figure}[h]
\begin{center}
  \includegraphics[width=\textwidth]{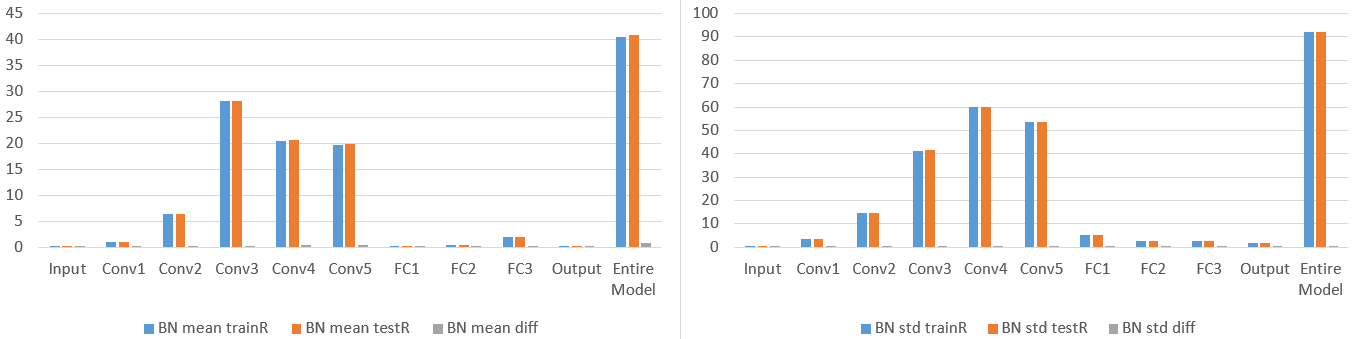}
\end{center}   
\caption{L2 norms of BN mean and standard deviation for dataset trainR and testR on Model MR, and their differences. Since it's trained and tested on the same dataset R, the differences (third bin in each layer) are relatively small.}
\label{fig:BN_ratio_RR}
\end{figure}


For comparison 2, we show the results in Table~\ref{tb:appdixA_exp2} and Fig~\ref{fig:BN_ratio_VV}. We can find although it's trained and tested on the same dataset V, the differences are relatively larger than those of R. This meets our expectation since \MADD{\vBase{}}{V}$=53.72\% <$ \MADD{\rBase{}}{\rBasen{}}$=88.36\%$.

\begin{table}[ht]
  \caption{L2 norms of BN mean and standard deviation for dataset trainV and testV on Model MV, and their differences. MA(MV, trainV)=84.82\%, MA(MV, testV)=53.72\%.}
  \label{tb:appdixA_exp2}
  \centering
  \scalebox{0.7}{
  \begin{tabular}{c|ccccccccccc}
    \toprule
    BN Position & Input & Conv1 & Conv2 & Conv3 & Conv4 & Conv5 & FC1 & FC2 & FC3 & Output & Model level\\
    \midrule
    mean trainV & 0.101 & 0.191 & 0.253 & 0.417 & 0.451 & 0.805 & 0.182 & 0.231 & 1.084 & 0.910 & 1.797 \\
    mean testV & 0.101 & 0.191 & 0.253 & 0.416 & 0.451 & 0.805 & 0.182 & 0.228 & 1.067 & 1.016 & 1.842 \\
    mean diff & 0.000 & 0.000 & 0.001 & 0.004 & 0.006 & 0.007 & 0.000 & 0.003 & 0.017 & 0.105 & 0.107 \\
    mean diff / mean trainV & 0.00\% & 0.00\% & 0.39\% & 0.96\% & 1.33\% & 0.87\% & 0.00\% & 1.30\% & 1.57\% & 11.54\% & 5.95\% \\
    \midrule
    std trainV & 0.368 & 0.494 & 0.946 & 1.451 & 1.605 & 2.007 & 0.520 & 1.217 & 3.295 & 3.817 & 6.097 \\
    std testV & 0.368 & 0.494 & 0.946 & 1.451 & 1.604 & 2.004 & 0.518 & 1.211 & 3.219 & 3.041 & 5.597 \\
    std diff & 0.000 & 0.000 & 0.000 & 0.003 & 0.004 & 0.009 & 0.002 & 0.006 & 0.075 & 0.776 & 0.779 \\
    std diff / std trainV & 0.00\% & 0.00\% & 0.00\% & 0.20\% & 0.25\% & 0.45\% & 0.38\% & 0.49\% & 2.28\% & 20.33\% & 12.788\% \\
    \bottomrule
  \end{tabular}
  }
\end{table}

\begin{figure}[h]
\begin{center}
  \includegraphics[width=\textwidth]{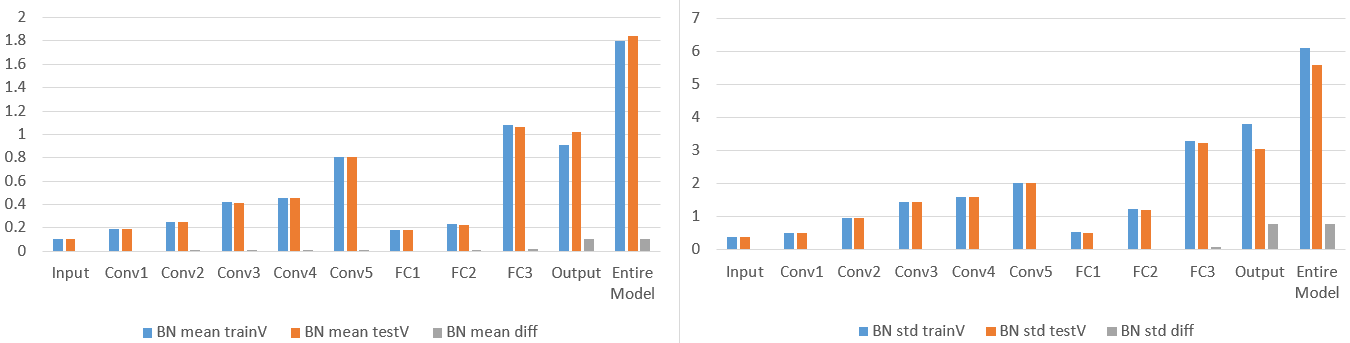}
\end{center}   
\caption{L2 norms of BN mean and standard deviation for dataset trainV and testV on Model MV, and their differences. We can find although it's trained and tested on the same dataset V, the differences (third bin of each layer) are relatively larger than those of R. This meets our expectation since \MADD{\vBase{}}{V}$=53.72\% <$ \MADD{\rBase{}}{\rBasen{}}$=88.36\%$.}
\label{fig:BN_ratio_VV}
\end{figure}

% \begin{table}[ht]
%   \caption{L2 norms of difference of standard deviations in $BN(MR, trainR)$ and $BN(MR, testR)$}
%   \label{tb:appdixA_exp1_std}
%   \centering
%   \scalebox{0.8}{
%   \begin{tabular}{c|ccccccccccc}
%     \toprule
%     BN Position & Input & Conv1 & Conv2 & Conv3 & Conv4 & Conv5 & FC1 & FC2 & FC3 & Output & Model level\\
%     \midrule
%     L2 norm & 0.001 & 0.009 & 0.032 & 0.115 & 0.229 & 0.433 & 0.018 & 0.010 & 0.007 & 0.136 & 0.662 \\
%     \bottomrule
%   \end{tabular}
%   }
% \end{table}


% \subsubsection{Experiment 2}
% Given a virtual simulator without any real dataset, we can have a model trained and tested just using the virtual dataset. This can give us $BN(MV, trainV)$ and $BN(MV, testV)$. Now, we want to deploy this trained model to a real car, which receives real data. Through the testing we now additionally have $BN(MV, R)$. We can first establish a baseline using the L2 norm between $BN(MV, trainV)$ and $BN(MV, testV)$, then use this baseline to contrast $BN(MV, V)$ (here $V$ can be either $trainV$ or $testV$) and $BN(MV, R)$. By doing this experiment, we can test the performance of the model trained on virtual data, but tested on both virtual data and real data, in order to find the difference of the virtual and real data on the virtually trained model. As a result, we get the DATASET difference on $MV$.

% Verify $BN(MV, trainV)$ is not similar with $BN(MV, testR)$. (V, R)

% Out of expectation. From Table \ref{tb:appdixA_exp2}, the mean differences are only slightly larger than those in experiment 1. But for standard deviation, only the first 3 layers are slightly larger than those in experiment 1, others are slightly smaller.


For comparison 3, we show the results in Table~\ref{tb:appdixA_exp3} and Fig~\ref{fig:BN_ratio_VR}. Since the model is tested on different dataset, we can find the BN statistics difference is much larger than those in comparison 1 and 2. Specifically, 103.80\% for mean and 22.10\% for std.

\begin{table}[ht]
  \caption{L2 norms of BN mean and standard deviation for dataset testV and testR on Model MV, and their differences. MA(MV, testV)=53.72\%, MA(MV, testR)=31.16\%.}
  \label{tb:appdixA_exp3}
  \centering
  \scalebox{0.7}{
  \begin{tabular}{c|ccccccccccc}
    \toprule
    BN Position & Input & Conv1 & Conv2 & Conv3 & Conv4 & Conv5 & FC1 & FC2 & FC3 & Output & Model level\\
    \midrule
    mean testV & 0.101 & 0.191 & 0.253 & 0.416 & 0.451 & 0.805 & 0.182 & 0.228 & 1.067 & 1.016 & 1.842 \\
    mean testR & 0.093 & 0.194 & 0.297 & 0.519 & 0.673 & 1.131 & 0.131 & 0.226 & 0.311 & 2.369 & 2.814 \\
    mean diff & 0.169 & 0.120 & 0.155 & 0.302 & 0.549 & 0.889 & 0.051 & 0.002 & 0.755 & 1.353 & 1.912 \\
    mean diff / mean testV & 167.33\% & 62.83\% & 61.26\% & 72.59\% & 121.73\% & 110.43\% & 28.02\% & 0.87\% & 70.76\% & 133.17\% & 103.80\% \\
    \midrule
    std testV & 0.368 & 0.494 & 0.946 & 1.451 & 1.604 & 2.004 & 0.518 & 1.211 & 3.219 & 3.041 & 5.597 \\
    std testR & 0.554 & 0.527 & 0.905 & 1.418 & 1.584 & 1.908 & 0.458 & 0.937 & 2.368 & 3.800 & 5.542 \\
    std diff & 0.195 & 0.125 & 0.166 & 0.166 & 0.133 & 0.156 & 0.059 & 0.273 & 0.851 & 0.758 & 1.237 \\
    std diff / std testV & 52.99\% & 25.30\% & 17.55\% & 11.44\% & 8.29\% & 7.78\% & 11.39\% & 22.54\% & 26.44\% & 24.93\% & 22.10\% \\
    \bottomrule
  \end{tabular}
  }
\end{table}

\begin{figure}[h]
\begin{center}
  \includegraphics[width=\textwidth]{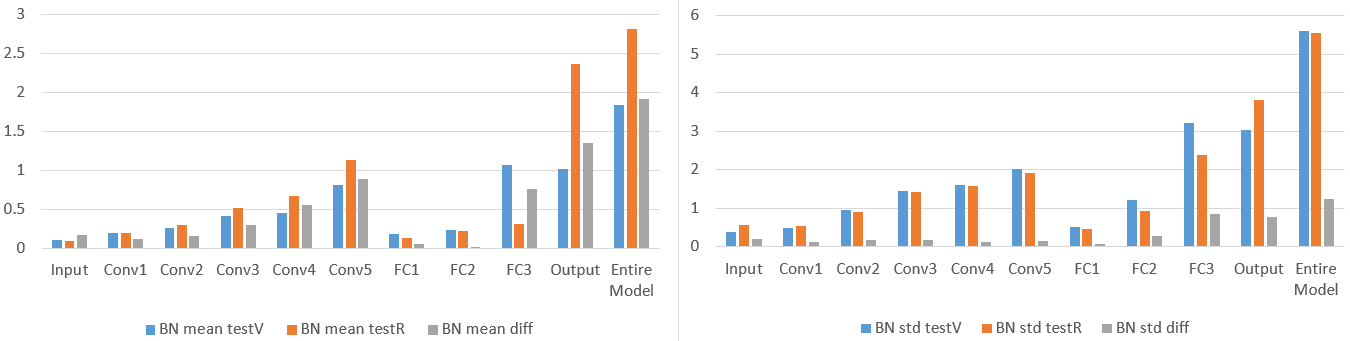}
\end{center}   
\caption{L2 norms of BN mean and standard deviation for dataset testV and testR on Model MV, and their differences. Since the model is tested on different dataset, we can find the BN statistics difference (third bin in ealy layer) is much larger than those in comparison 1 and 2.}
\label{fig:BN_ratio_VR}
\end{figure}



For comparison 4, we show the results in Table~\ref{tb:appdixA_exp4} and Fig~\ref{fig:BN_ratio_R1R1}.

\begin{table}[ht]
  \caption{L2 norms of BN mean and standard deviation for dataset trainR1 and testR1 on Model MR1, and their differences. MA(MR1, trainR1)=89.37\%, MA(MR1, testR1)=82.75\%.}
  \label{tb:appdixA_exp4}
  \centering
  \scalebox{0.7}{
  \begin{tabular}{c|ccccccccccc}
    \toprule
    BN Position & Input & Conv1 & Conv2 & Conv3 & Conv4 & Conv5 & FC1 & FC2 & FC3 & Output & Model level\\
    \midrule
    mean trainR1 & 0.285 & 1.086 & 3.989 & 7.815 & 4.613 & 4.107 & 0.226 & 0.019 & 1.351 & 0.178 & 10.87 \\
    mean testR1 & 0.284 & 1.083 & 3.978 & 7.796 & 4.619 & 4.041 & 0.226 & 0.019 & 1.350 & 0.142 & 10.83 \\
    mean diff & 0.001 & 0.003 & 0.012 & 0.069 & 0.092 & 0.166 & 0.000 & 0.000 & 0.001 & 0.036 & 0.206 \\
    mean diff / mean trainR1 & 0.35\% & 0.33\% & 0.31\% & 0.89\% & 2.00\% & 4.05\% & 0.07\% & 1.09\% & 0.04\% & 20.47\% & 1.89\% \\
    \midrule
    std trainR1 & 0.495 & 2.160 & 7.248 & 15.01 & 16.39 & 16.58 & 2.232 & 2.094 & 2.957 & 3.418 & 29.26 \\
    std testR1 & 0.496 & 2.163 & 7.248 & 15.01 & 16.40 & 16.59 & 2.222 & 2.080 & 2.950 & 3.402 & 29.27 \\
    std diff & 0.001 & 0.004 & 0.008 & 0.036 & 0.044 & 0.078 & 0.009 & 0.013 & 0.007 & 0.015 & 0.100 \\
    std diff / std trainR1 & 0.16\% & 0.18\% & 0.11\% & 0.24\% & 0.27\% & 0.47\% & 0.40\% & 0.66\% & 0.24\% & 0.46\% & 0.34\% \\
    \bottomrule
  \end{tabular}
  }
\end{table}

\begin{figure}[h]
\begin{center}
  \includegraphics[width=\textwidth]{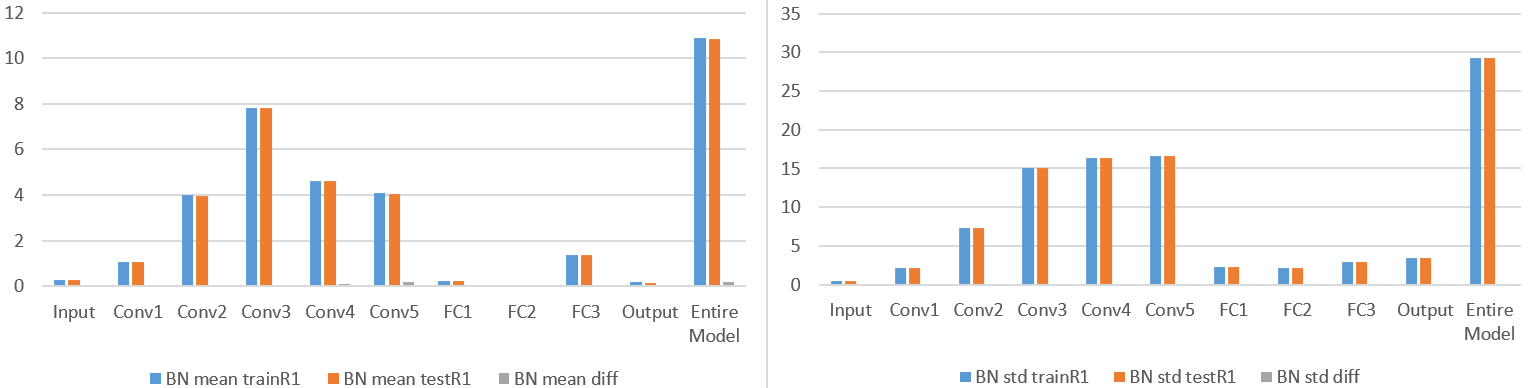}
\end{center}   
\caption{L2 norms of BN mean and standard deviation for dataset trainR1 and testR1 on Model MR1, and their differences. Since the model is tested on the same dataset, we can find the BN statistics difference (third bin in ealy layer) is small, similar with comparison 1.}
\label{fig:BN_ratio_R1R1}
\end{figure}


For comparison 5, we show the results in Table~\ref{tb:appdixA_exp5} and Fig~\ref{fig:BN_ratio_R1R}.

\begin{table}[ht]
  \caption{L2 norms of BN mean and standard deviation for dataset testR1 and testR on Model MR1, and their differences. MA(MR1, testR1)=82.75\%, MA(MR1, testR)=32.02\%.}
  \label{tb:appdixA_exp5}
  \centering
  \scalebox{0.7}{
  \begin{tabular}{c|ccccccccccc}
    \toprule
    BN Position & Input & Conv1 & Conv2 & Conv3 & Conv4 & Conv5 & FC1 & FC2 & FC3 & Output & Model level\\
    \midrule
    mean testR1 & 0.285 & 1.083 & 3.979 & 7.797 & 4.620 & 4.042 & 0.226 & 0.019 & 1.350 & 0.142 & 10.83 \\
    mean testR & 0.093 & 0.580 & 2.790 & 5.864 & 6.073 & 6.046 & 0.369 & 0.079 & 0.040 & 1.203 & 10.84 \\
    mean diff & 0.213 & 0.784 & 1.930 & 4.191 & 5.439 & 6.570 & 0.143 & 0.098 & 1.390 & 1.345 & 9.924 \\
    mean diff / mean testR1 & 74.94\% & 72.35\% & 48.51\% & 53.76\% & 117.74\% & 162.56\% & 63.12\% & 513.96\% & 102.93\% & 946.96\% & 91.57\% \\
    \midrule
    std testR1 & 0.496 & 2.163 & 7.248 & 15.01 & 16.41 & 16.59 & 2.223 & 2.081 & 2.950 & 3.402 & 29.27 \\
    std testR & 0.555 & 2.357 & 8.010 & 17.471 & 19.621 & 20.013 & 2.371 & 1.356 & 2.053 & 3.220 & 34.39 \\
    std diff & 0.064 & 0.326 & 1.156 & 3.648 & 5.459 & 5.082 & 0.148 & 0.725 & 0.898 & 0.182 & 8.472 \\
    std diff / std testR1 & 12.85\% & 15.07\% & 15.95\% & 24.29\% & 33.27\% & 30.62\% & 6.67\% & 34.84\% & 30.42\% & 5.36\% & 28.93\% \\
    \bottomrule
  \end{tabular}
  }
\end{table}

\begin{figure}[h]
\begin{center}
  \includegraphics[width=\textwidth]{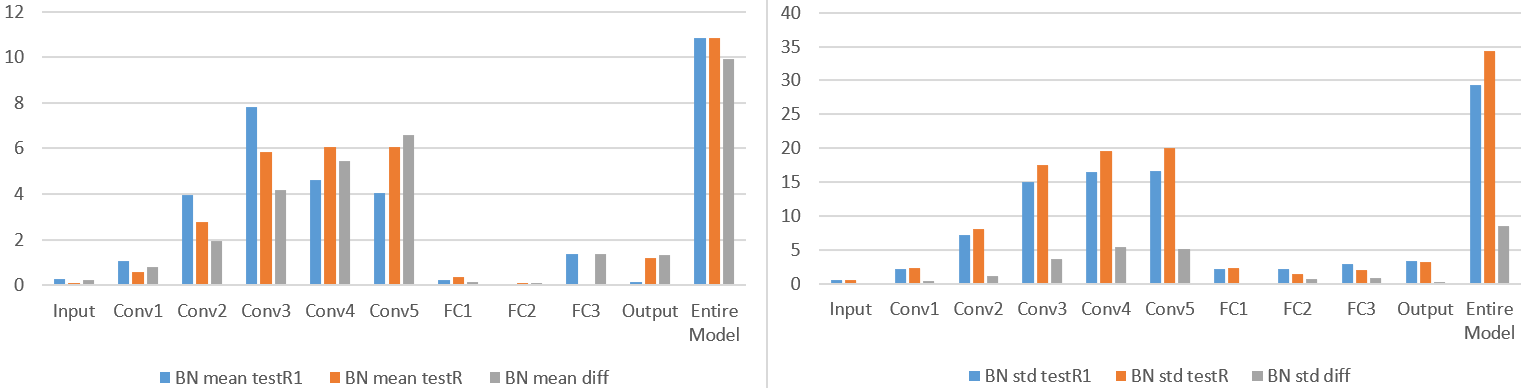}
\end{center}   
\caption{L2 norms of BN mean and standard deviation for dataset testR1 and testR on Model MR1, and their differences. Since the model is tested on different dataset, we can find the BN statistics difference (third bin in ealy layer) is much larger than those in comparison 1, 2, and 4, similar with comparison 3.}
\label{fig:BN_ratio_R1R}
\end{figure}


% % \begin{table}[ht]
% %   \caption{L2 norms of difference of standard deviations in $BN(MV, trainV)$ and $BN(MV, testR)$}
% %   \label{tb:appdixA_exp2_std}
% %   \centering
% %   \scalebox{0.8}{
% %   \begin{tabular}{c|ccccccccccc}
% %     \toprule
% %     BN Position & Input & Conv1 & Conv2 & Conv3 & Conv4 & Conv5 & FC1 & FC2 & FC3 & Output & Model level\\
% %     \midrule
% %     L2 norm & 0.195 & 0.125 & 0.166 & 0.166 & 0.133 & 0.156 & 0.062 & 0.280 & 0.927 & 0.017 & 1.181 \\
% %     \bottomrule
% %   \end{tabular}
% %   }
% % \end{table}


% \subsubsection{Experiment 3}
% Now, we have both virtual environment and real environment for our AVs. Using datasets in these two different domains, we can have $MV$ and $MR$. In real domain, we can establish the baseline as the difference between $BN(MR, trainR)$ and $BN(MR, testR)$. Now, we want to test how $MV$ performs in the real environment. As a result, we can have $BN(MV, R)$ (here $R$ can be either $trainR$ or $testR$). Using the difference between $BN(MV, R)$ and $BN(MR, R)$ (here $R$ can be either $trainR$ or $testR$) to contrast the baseline, we can have the MODEL difference not the DATASET difference, compared to Experiment 2. 



% Verify $BN(MV, testR)$ is not similar with $BN(MR, testR)$. (V, R) <-> (R, R)

% From Table \ref{tb:appdixA_exp3}, both mean and std are much larger than those in experiment 1.

% \begin{table}[h]
%   \caption{L2 norms of mean and standard deviation differences in $BN(MV, testR)$ and $BN(MR, testR)$}
%   \label{tb:appdixA_exp3}
%   \centering
%   \scalebox{0.8}{
%   \begin{tabular}{c|ccccccccccc}
%     \toprule
%     BN Position & Input & Conv1 & Conv2 & Conv3 & Conv4 & Conv5 & FC1 & FC2 & FC3 & Output & Model level\\
%     \midrule
%     mean & 0.000 & 0.967 & 6.270 & 27.90 & 20.48 & 20.11 & 0.425 & 0.166 & 1.554 & 2.463 & 40.64 \\
%     std & 0.000 & 2.998 & 13.96 & 40.30 & 58.82 & 51.80 & 4.666 & 1.548 & 0.226 & 2.196 & 89.45 \\
%     \bottomrule
%   \end{tabular}
%   }
% \end{table}

% \begin{table}[h]
%   \caption{L2 norms of difference of standard deviations in $BN(MV, testR)$ and $BN(MR, testR)$}
%   \label{tb:appdixA_exp3_std}
%   \centering
%   \scalebox{0.8}{
%   \begin{tabular}{c|ccccccccccc}
%     \toprule
%     BN Position & Input & Conv1 & Conv2 & Conv3 & Conv4 & Conv5 & FC1 & FC2 & FC3 & Output & Model level\\
%     \midrule
%     L2 norm & 0.000 & 2.998 & 13.96 & 40.30 & 58.82 & 51.80 & 4.666 & 1.548 & 0.226 & 2.196 & 89.45 \\
%     \bottomrule
%   \end{tabular}
%   }
% \end{table}


\subsection{Image Quality}
Here, we present the results that are related to image quality reduction of real images. The results associated with the blur effect is shown in Table~\ref{tab:bn_blur}.  

We calculate the \ltwo{ }norm of the \BN{} statistics between \BNDD{$R$}{\rBasen{}} (baseline) and \BNDD{\rBase{}}{D} (Table~\ref{tab:bn_blur}(a)) or \BNDD{$D$}{\rBasen{}} (Table~\ref{tab:bn_blur}(b)), where $D \in \{B1, B2, B3, B4, B5\}$, using the corresponding mean and standard deviation values, respectively. In both Table~\ref{tab:bn_blur}(a) and Table~\ref{tab:bn_blur}(b), we show the absolute mean accuracy (\MA{}) difference of \MADD{\rBase{}}{D} or \MADD{$D$}{\rBasen{}} to \MADD{$R$}{\rBasen{}} for comparison.

We find that as the \MA{} difference increases, the \ltwo{} norm of \MADD{\rBase{}}{D} or \MADD{$D$}{\rBasen{}} increases. In addition, changing the blur level of the training dataset will result in larger \ltwo{} norm than changing the blur level of the test dataset.

In Table~\ref{tab:bn_noise} and Table~\ref{tab:bn_distortion}, we show the results associated with the noise effect and the distortion effect, respectively. For the noise effect, when increasing the noise level of the test set (Table~\ref{tab:bn_noise}(a)), the \ltwo{} norm increases as the absolute \MA{} difference increases. However, the same phenomenon is not found when increasing the noise level of the training dataset (Table~\ref{tab:bn_noise}(b)). For the distortion effect, similar behaviors are observed. In addition, for both effects, changing the intensity level of the effect on the training dataset will result in larger \ltwo{} values than changing that of the test dataset. 



\begin{table}[ht]
      \centering
      \caption{\BN{} statistics results of the blur effect. The \ltwo{} norm of \BNDD{\rBase{}}{D} and \BNDD{$D$}{\rBasen{}} to the baseline \BNDD{$R$}{\rBasen{}}, using the corresponding mean and standard deviation values are reported. In both (a) and (b), the absolute \MA{} difference is also shown for comparison. Overall, we find the \ltwo{} norm values correlate positively with the \MA{} difference. In addition, changing the blur level of the training dataset has higher influence on \ltwo{} norm than changing the blur level of the test dataset. Given $\|$\BNDDC{\rBase{}}{\rBasen{}}{mean}$\|_2=40.08$, $\|$\BNDDC{\rBase{}}{\rBasen{}}{std}$\|_2=92.04$, and \MADD{\rBase{}}{\rBasen{}} $=88.36\%$.}      
      
      \begin{tabular}{cl|cccccc}
        \toprule
         & & &  \multicolumn{3}{c}{ Dataset ($D$)} \\
         & & $B1$ & $B2$ & $B3$ & $B4$ & $B5$\\
        \midrule
        & $\|$\BNDDC{\rBase{}}{D}{mean}$\|_2$ & 40.77 & 40.69 & 40.31 & 39.77 & 39.51 \\
        & $\|$\BNDDC{\rBase{}}{D}{mean} $-$ \BNDDC{\rBase{}}{\rBasen{}}{mean}$\|_2$ & 0.10 & 0.99 & 3.65 & 3.45 & 7.87 \\
        & $\Delta$\BNDDC{\rBase{}}{}{mean} $/$ $\|$
        \BNDDC{\rBase{}}{\rBasen{}}{mean}$\|_2$ & 0.23\% & 2.44\% & 8.93\% & 8.45\% & 19.29\% \\
        \cmidrule(r){2-7}
        & $\|$\BNDDC{\rBase{}}{D}{std}$\|_2$ & 91.91 & 91.87 & 88.20 & 86.17 & 79.66 \\
    (a) & $\|$\BNDDC{\rBase{}}{D}{std} $-$ \BNDDC{\rBase{}}{\rBasen{}}{std}$\|_2$ & 0.18 & 0.58 & 4.26 & 7.50 & 14.63 \\
        & $\Delta$\BNDDC{\rBase{}}{}{std} $/$ $\|$ \BNDDC{\rBase{}}{\rBasen{}}{std}$\|_2$ & 0.19\% & 0.62\% & 4.63\% & 8.14\% & 15.88\% \\
        \cmidrule(r){2-7}
        & \MADD{\rBase{}}{D}  & 88.21\% & 88.06\% & 86.07\% & 81.16\% & 73.33\% \\
        & $|$\MADD{\rBase{}}{D} $-$ \MADD{\rBase{}}{\rBasen{}}$|$ & 0.15\% & 0.3\% & 2.29\% & 7.2\% & 15.03\% \\
        & $\Delta$\MADD{\rBase{}}{} $/$ \MADD{\rBase{}}{\rBasen{}} & 0.17\% & 0.34\% & 2.59\% & 8.15\% & 17.01\% \\
        \midrule
        %Element & (B1, R) & (B2, R) & (B3, R) & (B4, R) & (B5, R)\\
        %\midrule
        & $\|$\BNDDC{$D$}{D}{mean}$\|_2$ & 30.34 & 43.39 & 42.23 & 41.24 & 46.63 \\
        & $\|$\BNDDC{$D$}{\rBasen{}}{mean}$\|_2$ & 30.37 & 43.65 & 42.43 & 42.43 & 48.80 \\
        & $\|$\BNDDC{$D$}{D}{mean} $-$ \BNDDC{$D$}{\rBasen{}}{mean}$\|_2$ & 0.08 & 1.18 & 4.18 & 3.05 & 9.15 \\
        & $\Delta$\BNDDC{$D$}{}{mean} $/$ $\|$ \BNDDC{$D$}{D}{mean}$\|_2$  & 0.27\% & 2.73\% & 9.90\% & 7.40\% & 19.62\% \\
        \cmidrule(r){2-7}
        & $\|$\BNDDC{$D$}{D}{std}$\|_2$ & 71.46 & 100.61 & 96.70 & 100.87 & 107.85 \\
    (b) & $\|$\BNDDC{$D$}{\rBasen{}}{std}$\|_2$ & 71.58 & 100.49 & 100.54 & 105.38 & 121.52 \\
        & $\|$\BNDDC{$D$}{D}{std} $-$ \BNDDC{$D$}{\rBasen{}}{std}$\|_2$ & 0.16 & 0.50 & 4.09 & 5.61 & 16.02 \\
        & $\Delta$\BNDDC{$D$}{}{std} $/$ $\|$ \BNDDC{$D$}{D}{std}$\|_2$ & 0.22\% & 0.50\% & 4.23\% & 5.56\% & 14.85\% \\
        \cmidrule(r){2-7}
        & \MADD{$D$}{D} & 87.08\% & 89.34\% & 87.70\% & 87.64\% & 88.51\% \\
        & \MADD{$D$}{\rBasen{}} & 87.05\% & 89.10\% & 86.16\% & 82.58\% & 76.45\% \\
        & $|$\MADD{$D$}{D} $-$ \MADD{$D$}{\rBasen{}}$|$  & 0.03\% & 0.24\% & 1.54\% & 5.06\% & 12.06\% \\
        & $\Delta$\MADD{$D$}{} $/$ \MADD{$D$}{D} & 0.03\% & 0.26\% & 1.75\% & 5.77\% & 13.62\% \\
        \bottomrule
      \end{tabular}
      \label{tab:bn_blur}
\end{table}
   %   We calculate the L2 norm of the BN statistics difference between \BNMD{$train(R)$}{\rBasen{}} (baseline) and \BNDD{\rBase{}}{D} / \BNDD{$D$}{\rBasen{}}, where $D \in \{B1, B2, B3, B4, B5\}$, and show L2 norm of mean difference and std difference in second row and third row, respectively. In the forth row, we show the absolute Mean Accuracy (\MA{}) difference between \MAMD{$train(R)$}{\rBasen{}} (baseline) and \MADD{\rBase{}}{D} / \MADD{$D$}{\rBasen{}}, where $D \in \{B1, B2, B3, B4, B5\}$. We can find no matter we increase the blur level of test dataset (upper part) or training dataset (bottom part), the L2 norm of Mean diff and Std diff increase with the increasing of the \MA{} diff, showing that they are positive related. In addition, changing the blur level of the training dataset will have larger BN mean and std differences than changing the blur level of the test dataset.


\begin{figure}[h]
\begin{center}
  \includegraphics[width=\textwidth]{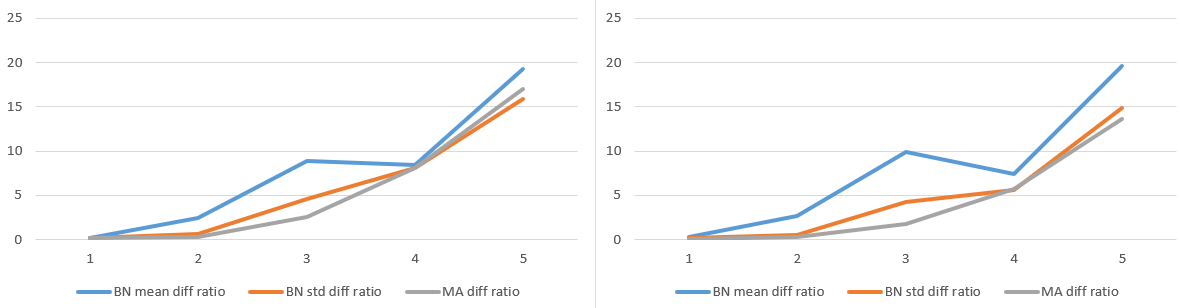}
\end{center}   
\caption{Curve for blur. Showing the MA percentage difference is nearly positive related to the the BN statistics percentage difference, including mean and std.}
\label{fig:BN_ratio_blur}
\end{figure}



\begin{table}[ht]
      \centering
      \caption{\BN{} statistics results of the noise effect. The \ltwo{} norm of \MADD{\rBase{}}{D} and \MADD{$D$}{\rBasen{}} to the baseline \BNDD{$R$}{\rBasen{}}, using the corresponding mean and standard deviation values are reported. In both (a) and (b), the absolute \MA{} difference is also shown for comparison. We find that when increasing the noise level of test dataset (a), the \ltwo{} norm increases as the absolute \MA{} difference increases. However, when increasing the noise level of the training dataset (b), similar behavior is not found. In addition, changing the noise level of the training dataset will result in larger \ltwo{} norm than changing the test dataset.}
      \begin{tabular}{cl|cccccc}
        \toprule
        & & &  \multicolumn{3}{c}{ Dataset ($D$)} \\
        & & $N1$ & $N2$ & $N3$ & $N4$ & $N5$\\
        \midrule
        & $\|$\BNDDC{\rBase{}}{D}{mean}$\|_2$ & 39.89 & 37.25 & 31.18 & 26.06 & 22.66 \\
        & $\|$\BNDDC{\rBase{}}{D}{mean} $-$ \BNDDC{\rBase{}}{\rBasen{}}{mean}$\|_2$ & 1.65 & 4.86 & 10.57 & 15.85 & 19.74 \\
        & $\Delta$\BNDDC{\rBase{}}{}{mean} $/$ $\|$
        \BNDDC{\rBase{}}{\rBasen{}}{mean}$\|_2$ & 4.05\% & 11.91\% & 25.92\% & 38.84\% & 48.37\% \\
        \cmidrule(r){2-7}
        & $\|$\BNDDC{\rBase{}}{D}{std}$\|_2$ & 90.49 & 85.33 & 72.06 & 60.03 & 51.10 \\
    (a) & $\|$\BNDDC{\rBase{}}{D}{std} $-$ \BNDDC{\rBase{}}{\rBasen{}}{std}$\|_2$ & 1.62 & 6.79 & 20.04 & 32.10 & 41.05 \\
        & $\Delta$\BNDDC{\rBase{}}{}{std} $/$ $\|$ \BNDDC{\rBase{}}{\rBasen{}}{std}$\|_2$ & 1.76\% & 7.37\% & 21.77\% & 34.87\% & 44.60\% \\
        \cmidrule(r){2-7}
        & \MADD{\rBase{}}{D}  & 88.33\% & 86.01\% & 81.42\% & 76.39\% & 73.15\% \\
        & $|$\MADD{\rBase{}}{D} $-$ \MADD{\rBase{}}{\rBasen{}}$|$ & 0.03\% & 2.35\% & 6.94\% & 11.97\% & 15.21\% \\
        & $\Delta$\MADD{\rBase{}}{} $/$ \MADD{\rBase{}}{\rBasen{}} & 0.03\% & 2.65\% & 7.85\% & 13.54\% & 17.21\% \\
        \midrule
        %Element & (B1, R) & (B2, R) & (B3, R) & (B4, R) & (B5, R)\\
        %\midrule
        & $\|$\BNDDC{$D$}{D}{mean}$\|_2$ 
        & 41.56 & 35.01 & 1.61 & 1.39 & 0.66 \\
        & $\|$\BNDDC{$D$}{\rBasen{}}{mean}$\|_2$ 
        & 42.50 & 38.24 & 2.18 & 2.01 & 1.04 \\
        & $\|$\BNDDC{$D$}{D}{mean} $-$ \BNDDC{$D$}{\rBasen{}}{mean}$\|_2$ 
        & 1.48 & 4.24 & 0.69 & 0.80 & 0.53 \\
        & $\Delta$\BNDDC{$D$}{}{mean} $/$ $\|$ \BNDDC{$D$}{D}{mean}$\|_2$  
        & 3.56\% & 12.13\% & 43.02\% & 57.99\% & 80.43\% \\
        \cmidrule(r){2-7}
        & $\|$\BNDDC{$D$}{D}{std}$\|_2$ 
        & 84.71 & 82.68 & 4.86 & 2.95 & 1.89 \\
    (b) & $\|$\BNDDC{$D$}{\rBasen{}}{std}$\|_2$ 
        & 86.23 & 89.69 & 6.36 & 4.56 & 2.60 \\
        & $\|$\BNDDC{$D$}{D}{std} $-$ \BNDDC{$D$}{\rBasen{}}{std}$\|_2$ 
        & 1.59 & 7.11 & 1.54 & 1.71 & 0.98 \\
        & $\Delta$\BNDDC{$D$}{}{std} $/$ $\|$ \BNDDC{$D$}{D}{std}$\|_2$ 
        & 1.88\% & 8.60\% & 31.72\% & 58.03\% & 51.98\% \\
        \cmidrule(r){2-7}
        & \MADD{$D$}{D} 
        & 88.45\% & 87.35\% & 66.22\% & 60.17\% & 54.34\% \\
        & \MADD{$D$}{\rBasen{}} 
        & 89.1\% & 86.57\% & 66.63\% & 58.24\% & 53.83\% \\
        & $|$\MADD{$D$}{D} $-$ \MADD{$D$}{\rBasen{}}$|$  
        & 0.65\% & 0.78\% & 0.41\% & 1.93\% & 0.51\% \\
        & $\Delta$\MADD{$D$}{} $/$ \MADD{$D$}{D} 
        & 0.73\% & 0.89\% & 0.61\% & 3.20\% & 0.93\% \\
        \bottomrule
      \end{tabular}
      \label{tab:bn_noise}
\end{table}


\begin{figure}[h]
\begin{center}
  \includegraphics[width=\textwidth]{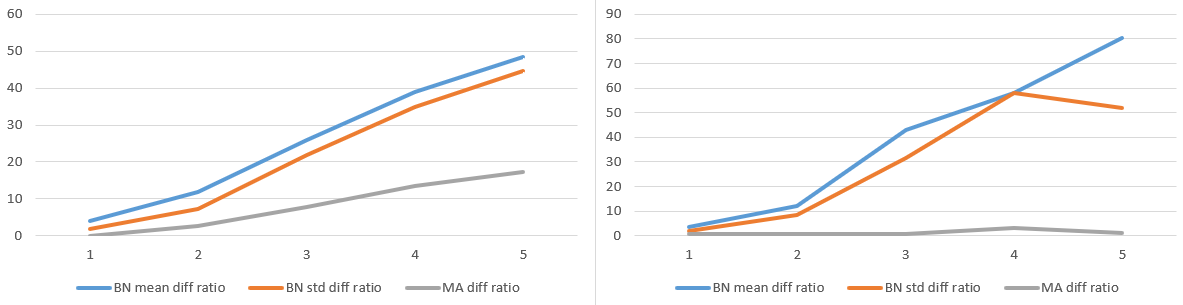}
\end{center}   
\caption{Curve for noise. Showing the MA percentage difference is nearly positive related to the the BN statistics percentage difference, including mean and std.}
\label{fig:BN_ratio_noise}
\end{figure}


\begin{table}[ht]
      \centering
      \caption{\BN{} statistics results of the distortion effect. The \ltwo{} norm of \MADD{\rBase{}}{D} and \MADD{$D$}{\rBasen{}} to the baseline \BNDD{$R$}{\rBasen{}}, using the corresponding mean and standard deviation values are reported. In both (a) and (b), the absolute \MA{} difference is also shown for comparison. We find that when increasing the distortion level of test dataset (a), the \ltwo{} norm increases as the absolute \MA{} difference increases. However, when increasing the distortion level of the training dataset (b), similar behavior is not shown. In addition, changing the distortion level of the training dataset will result in larger \ltwo{} norm than changing the test dataset.}
      \begin{tabular}{cl|cccccc}
        \toprule
        & & &  \multicolumn{3}{c}{ Dataset ($D$)} \\
        & & D1 & D2 & D3 & D4 & D5\\
        \midrule
        & $\|$\BNDDC{\rBase{}}{D}{mean}$\|_2$ & 40.73 & 45.78 & 71.29 & 97.46 & 110.20 \\
        & $\|$\BNDDC{\rBase{}}{D}{mean} $-$ \BNDDC{\rBase{}}{\rBasen{}}{mean}$\|_2$ & 1.04 & 18.12 & 53.76 & 83.17 & 97.09 \\
        & $\Delta$\BNDDC{\rBase{}}{}{mean} $/$ $\|$
        \BNDDC{\rBase{}}{\rBasen{}}{mean}$\|_2$ & 2.55\% & 44.40\% & 131.74\% & 203.81\% & 237.91\% \\
        \cmidrule(r){2-7}
        & $\|$\BNDDC{\rBase{}}{D}{std}$\|_2$ & 91.77 & 90.20 & 87.01 & 73.25 & 61.92 \\
    (a) & $\|$\BNDDC{\rBase{}}{D}{std} $-$ \BNDDC{\rBase{}}{\rBasen{}}{std}$\|_2$ & 0.45 & 5.85 & 15.68 & 26.01 & 35.92 \\
        & $\Delta$\BNDDC{\rBase{}}{}{std} $/$ $\|$ \BNDDC{\rBase{}}{\rBasen{}}{std}$\|_2$ & 0.48\% & 6.35\% & 17.04\% & 28.26\% & 39.03\% \\
        \cmidrule(r){2-7}
        & \MADD{\rBase{}}{D}  & 88.63\% & 74.97\% & 57.67\% & 48.83\% & 49.16\% \\
        & $|$\MADD{\rBase{}}{D} $-$ \MADD{\rBase{}}{\rBasen{}}$|$ & 0.27\% & 13.39\% & 30.69\% & 39.53\% & 39.2\% \\
        & $\Delta$\MADD{\rBase{}}{} $/$ \MADD{\rBase{}}{\rBasen{}} & 0.30\% & 15.15\% & 34.73\% & 44.73\% & 44.36\% \\
        \midrule
        %Element & (B1, R) & (B2, R) & (B3, R) & (B4, R) & (B5, R)\\
        %\midrule
        & $\|$\BNDDC{$D$}{D}{mean}$\|_2$ 
        & 28.42 & 37.90 & 42.30 & 32.86 & 25.60 \\
        & $\|$\BNDDC{$D$}{\rBasen{}}{mean}$\|_2$ 
        & 28.44 & 34.59 & 31.02 & 30.38 & 23.18 \\
        & $\|$\BNDDC{$D$}{D}{mean} $-$ \BNDDC{$D$}{\rBasen{}}{mean}$\|_2$ 
        & 0.68 & 11.31 & 29.21 & 28.22 & 28.22 \\
        & $\Delta$\BNDDC{$D$}{}{mean} $/$ $\|$ \BNDDC{$D$}{D}{mean}$\|_2$  
        & 2.39\% & 29.85\% & 69.06\% & 85.87\% & 110.23\% \\
        \cmidrule(r){2-7}
        & $\|$\BNDDC{$D$}{D}{std}$\|_2$ 
        & 63.15 & 79.72 & 67.69 & 43.47 & 28.83 \\
    (b) & $\|$\BNDDC{$D$}{\rBasen{}}{std}$\|_2$ 
        & 63.31 & 80.88 & 76.00 & 61.05 & 51.97 \\
        & $\|$\BNDDC{$D$}{D}{std} $-$ \BNDDC{$D$}{\rBasen{}}{std}$\|_2$ 
        & 0.31 & 3.94 & 11.40 & 19.51 & 25.42 \\
        & $\Delta$\BNDDC{$D$}{}{std} $/$ $\|$ \BNDDC{$D$}{D}{std}$\|_2$ 
        & 0.49\% & 4.94\% & 16.85\% & 44.87\% & 88.19\% \\
        \cmidrule(r){2-7}
        & \MADD{$D$}{D} 
        & 88.92\% & 89.01\% & 86.36\% & 86.51\% & 85.83\% \\
        & \MADD{$D$}{\rBasen{}} 
        & 88.6\% & 75.56\% & 61.1\% & 54.49\% & 42.97\% \\
        & $|$\MADD{$D$}{D} $-$ \MADD{$D$}{\rBasen{}}$|$  
        & 0.32\% & 13.45\% & 25.26\% & 32.02\% & 42.86\% \\
        & $\Delta$\MADD{$D$}{} $/$ \MADD{$D$}{D} 
        & 0.36\% & 15.11\% & 29.25\% & 37.01\% & 49.93\% \\
        \bottomrule
      \end{tabular}
      \label{tab:bn_distortion}
\end{table}

\begin{figure}[h]
\begin{center}
  \includegraphics[width=\textwidth]{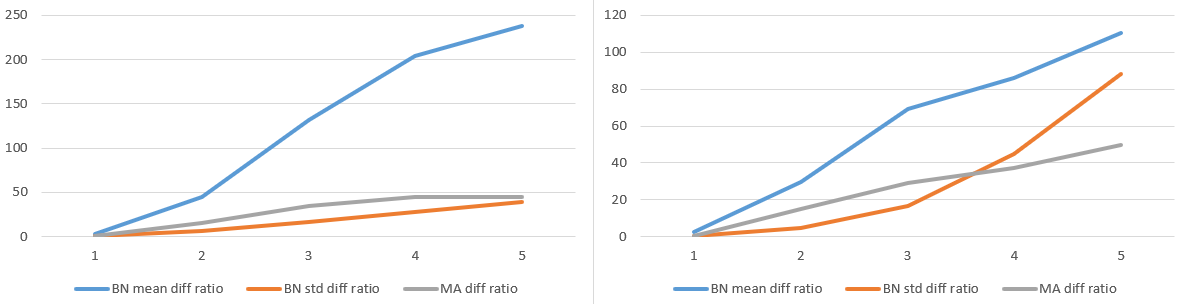}
\end{center}   
\caption{Curve for distortion. Showing the MA percentage difference is nearly positive related to the the BN statistics percentage difference, including mean and std.}
\label{fig:BN_ratio_distortion}
\end{figure}


\begin{figure}[h]
\begin{center}
  \includegraphics[width=\textwidth]{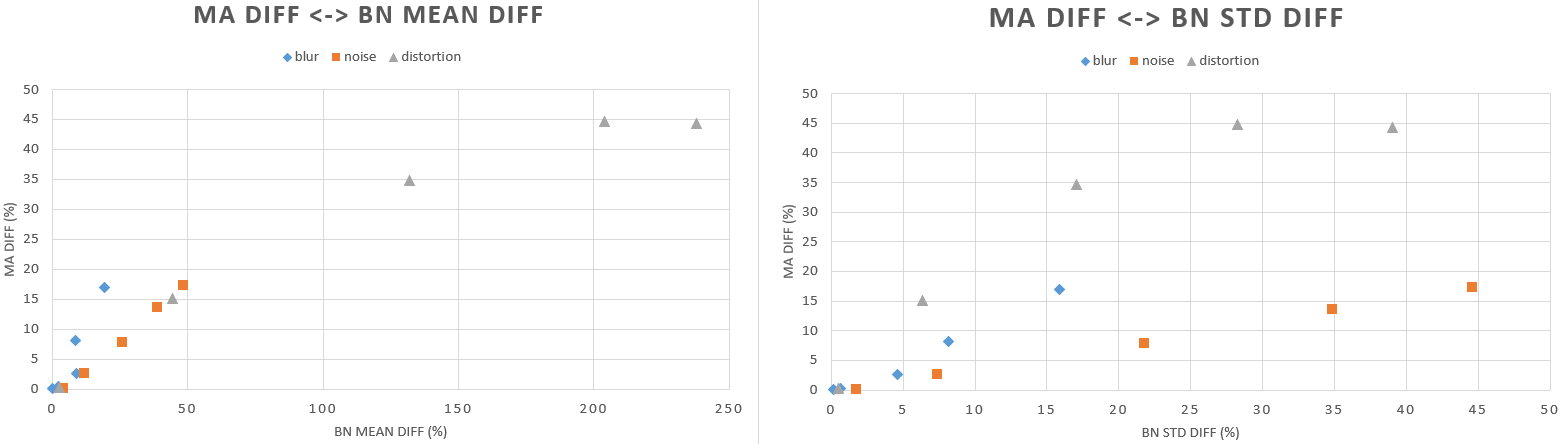}
\end{center}   
\caption{Data points, showing the relationship between MA percentage difference and BN statistics percentage difference. Overall, the trend of different factor look different (only the noise and distortion factor have similar trend in the left figure). }
\label{fig:BN_ratio_distortion}
\end{figure}


\begin{figure}[h]
\begin{center}
  \includegraphics[width=\textwidth]{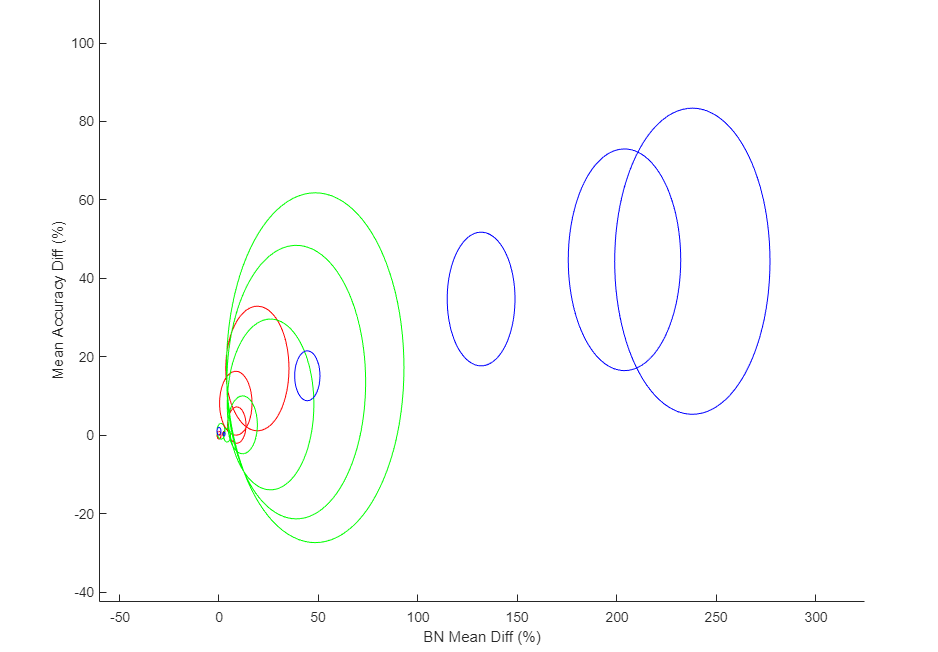}
\end{center}   
\caption{Data points, showing the relationship between MA percentage difference and BN statistics percentage difference. Red circles are "blur" factor, green circles are "noise" factor, blue circles are "distortion" factor. }
\label{fig:BN_ratio_distortion}
\end{figure}

% \subsection{Image style}
% Here, we present in Table~\ref{tb:bn_style} the results regarding image style. We use \BNDD{$R$}{\rBasen{}} as the baseline. Overall, we find no clear relationships between the \BN{} statistics difference and the \MA{} difference. 

% \begin{table}[ht]
%   \caption{\BN{} statistics results of different image styles and training strategies. We use \BNDD{$R$}{\rBasen{}} as the baseline, and calculate the \ltwo{} norm of mean/std difference between the baseline and \BNMDC{$M$}{\rBasen{}}{} for different model $M$. We use notations $\Delta \rm{BN}^{mean}=\|$\BNMDC{$M$}{\rBasen{}}{mean} $-$ \BNDDC{\rBase{}}{\rBasen{}}{mean}$\|_2$, $\Delta \rm{BN}^{std}=\|$\BNMDC{$M$}{\rBasen{}}{std} $-$ \BNDDC{\rBase{}}{\rBasen{}}{std}$\|_2$, and $\Delta \rm{MA}=|$\MAMD{$M$}{\rBasen{}} $-$ \MADD{$D$}{\rBasen{}}$|$. 
%   In general, we find no clear correlations between between the \BN{} statistics difference and the \MA{} difference.}
%   \label{tb:bn_style}
%   \centering
%   \scalebox{1.0}{
%   \begin{tabular}{l|c|c|c|c|c|c|c}
%     \toprule
%     & Model $M$ & $\Delta \rm{MA}$ & $\Delta \rm{MA} \%$ & $\Delta \rm{BN}^{mean}$ & $\Delta \rm{BN}^{mean} \%$ & $\Delta \rm{BN}^{std}$ & $\Delta \rm{BN}^{std} \%$ \\
%     \midrule
%         %& \train(\rBase{}) & 88.36\%\\
%          & \train(\vBase{}) & 57.2\% & xxx\% & 40.64 & xxx\% & 89.44 & xxx\%\\
% (a) Single  & \train(\vrgan{}) & 61.49\% & xxx\% & 36.33 & xxx\% & 59.26 & xxx\%\\
%         dataset & \train(\vrmunit{}) & 62.8\% & xxx\% & 35.65 & xxx\% & 48.37 & xxx\%\\
          
%     \midrule
%           &\train(\vBase{} + \rBase{}) & 11.34\% & xxx\% & 39.58 & xxx\% & 74.41 & xxx\%\\
% (b) Simply  & \train(\vrgan{} + \rBase{})  & 12.92\% & xxx\% & 38.67 & xxx\% & 53.41 & xxx\%\\
%           combine &\train(\vrmunit{} + \rBase{}) & 11.51\% & xxx\% & 37.49 & xxx\% & 74.85 & xxx\%\\
%     \midrule
%           & \pretrainTrain{\vBase{}}{\rBase{}} & 4.82\% & xxx\% & 36.67 & xxx\% & 76.31 & xxx\%\\
% (c) Pretrain +  & \pretrainTrain{\vrgan{}}{\rBase{}} & 5.66\% & xxx\% & 57.55 & xxx\% & 74.80 & xxx\%\\
%           retrain & \pretrainTrain{\vrmunit{}}{\rBase{}} & 9.32\% & xxx\% & 42.03 & xxx\% & 58.97 & xxx\%\\
%     \midrule
%           & \pretrainPartialRetrain{\vBase{}}{\rBase{}} & 14.7\% & xxx\% & 40.19 & xxx\% & 86.20 & xxx\%\\
% (d) Pretrain +  & \pretrainPartialRetrain{\vrgan{}}{\rBase{}} & 11.19\% & xxx\% & 37.63 & xxx\% & 59.93 & xxx\%\\
%           partially retrain & \pretrainPartialRetrain{\vrmunit{}}{\rBase{}} & 15.39\% & xxx\% & 35.62 & xxx\% & 48.26 & xxx\%\\
%     \bottomrule
%   \end{tabular}
%   }
% \end{table}


\clearpage
